# Supplementary material for: Linear Stability Analysis of Compressible Channel Flow with Porous Walls
Source: arXiv:1509.03152 source file (2015-12-27)
Supplement: Supplementary file 1 [file Appendix.tex]

%!TEX root = RahbariScalo_WhitherTurbulence_2015.tex
\section{Appendix}
\label{sec:App}
